# Supplementary material for: Library of efficient algorithms for phylogenetic analysis
Source: arXiv:2012.12697 source file (2020-12-30)
Supplement: Supplementary file 1 [file appendix.tex]

\begin{appendices}
\chapter*{Appendix A}
The contents...

\chapter*{Appendix B}
The contents...
\end{appendices}
